# Supplementary material for: Universality of the {\bf q}=1/2 Orbital Magnetism in the Pseudogap Phase of the High-$T_c$ superconductor $\rm YBa_{2}Cu_{3}O_{6+x}$
Source: arXiv:2302.01870 source file (2023-11-26)
Supplement: Supplementary file 1 [file Supple-nov23-arxiv.pdf]

**Supplementary information: Universality of the q=1/2 Orbital Magnetism in the Pseudogap Phase of the High-$T_c$ superconductor** $\mathrm{YBa_2Cu_3O_{6+x}}$

## 1 Polarized Neutron Diffraction

The polarized neutron measurements were performed on two different neutron Triple Axis Spectrometers: 4F1 at LLB-Orphée reactor in Saclay (France) with final neutron wavevector $k_f = 2.57\text{Å}^{-1}$ and THALES at Institut Laue Langevin (ILL) in Grenoble (France) with $k_f = 1.5\text{Å}^{-1}$. On Thales, the Heusler monochromateur and analyser was double focused, with variable horizontal and fixed vertical focusing (optimized for $k_f = 1.5\text{Å}^{-1}$) for these diffraction experiments. Distances are 200cm fromm monochromateur to sample, and 123cm from sample to analyzer. On 4F1, the large Heusler analyser was focussed horizontally but not vertically. No collimators were used on neither instrument. The YBCO69 sample mosaic was about $\sim$ 1.9 deg. The YBCO6.9 sample and the quartz specimen have similar size and parallepipedal shape with a total volume of $\sim$ 1 cm$^3$.

The flipping ratios (FR) have been measured on both the YBCO69 sample and on a quartz specimen. The Fig. S1 represents the flipping ratios measured on a quartz specimen on Thales over the **Q**-range of the measurement reported in Fig. 2 of the manuscript. A FR of about 37 is found on the quartz specimen with error bars given in Fig. S1. They vary in Q as the intensity of quartz exhibit a maximum in Q. On THALES, the flipping ratios have been measured as well on the (1,0,0) Bragg peak of the YBCO69 sample: FR $\sim$ 41.3$\pm$ 0.6 along the X direction ($\equiv$ Q direction), FR $\sim$ 39.1$\pm$ 0.6 along the Y direction and FR $\sim$ 40.9$\pm$ 0.6 along the Z direction (perpendicular to the scattering plane). On 4F1, the flipping ratios also measured on the (1,0,0) Bragg peak of the YBCO69 sample are found as FR $\sim$ 15$\pm$ 0.1 along the X direction, FR $\sim$ 15$\pm$ 0.1 along the Y direction and FR $\sim$ 15.2$\pm$ 0.2 along the Z direction. From these polarization XYZ-dependence of FR, one can notice on both instruments tiny variations of the polarization depending on its direction.

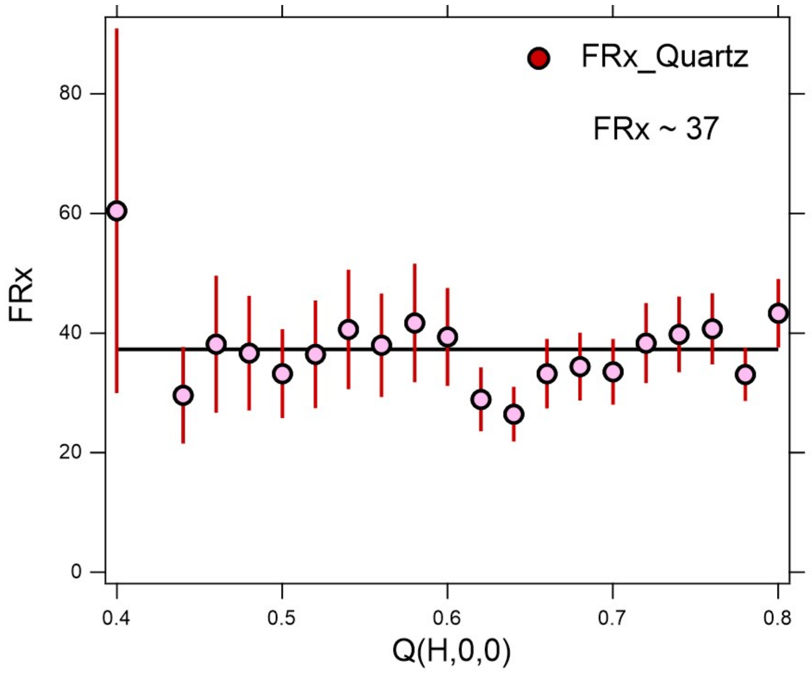


Supplementary Figure S1: Flipping ratio measured on a quartz specimen (Thales). For a sake of comparison, the wavevector of the figure is given in the reduced lattice units of YBCO69 sample: Q=$2\pi/a$H with $a$=3.85 Å.

The Fig. S2 shows the non-spin-flip (NSF) measurement in the YBCO69 sample for the **X** polarization for the same scan as the measurement in the spin-flip (SF) channel reported in Fig. 2d of the manuscript. No peak is seen in the NSF channel in contrast to the SF channel. This is consistent with the orthorhombic I phase where no signal from chains are present at H=1/2 contrary the ortho-II phase that exists at lower dopings. The shape of the NSF actually ressembles to the background shape of the SF channel. As the signal is here featureless in the non-spin-flip channel, the corrections from imperfect neutron polarization are marginal and would only affect the detailed shape of the background. The blue area in the lower panel represents the product of the magnetic signal times the instrumental flipping ratio measured on the quartz specimen (Fig. S1). That shows how much should be present in the NSF channel to give rise to a contamination in the SF channel due polarization leakage. This is clearly not the case in the measurement.

The FR$\sim$ 37 measured in the Quartz (Fig. S1) is more representative as the

observed magnetic peak is significantly broader than the Bragg resolution. It is further measured for the same wavevectors as the magnetic peaks in YBCO69. If one takes the FR $\sim$ 41 of the Bragg peak of the sample, the blue peak in Fig. S2 would be even larger.

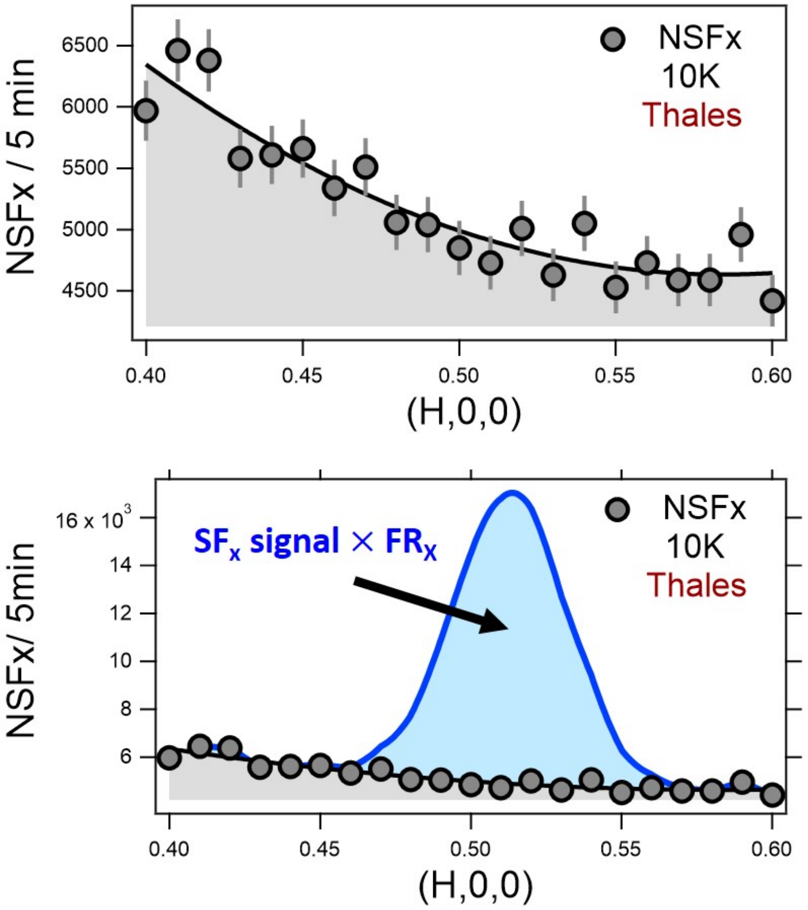


Supplementary Figure S2: Neutron intensity measured in the YBCO69 sample on Thales in the non-spin-flip channel for the **X** polarization (see text).

## 2 Crystal growth and CuO impurities

After the submission of our manuscript, it was raised by one referee that the magnetic signal in the YBCO69 sample may come from powder inclusions of antiferromagnetic tenorite (CuO) impurities. First of all, CuO is antiferromagnetic (AF) [1, 2] with an ordered moment of 0.65 $\mu_B$ and $T_N$ =230 K. The

(1/2,0,-1/2) AF peak of CuO has a $|Q|$ very close to the (0.5,0,L) positions of YBCO69 that we have studied. Fig. S3 describes such a possible CuO magnetic powder line contribution into the (H,0,L) reciprocal plane used in our experiments. Fig. S3.a shows a general view where one can recognize in blue the Ewald sphere of a possible CuO powder contamination that is crossing the (1/2,0,L) direction of YBCO reciprocal space as it is zoomed in Fig. S3.b. Therefore, it is important to address this issue. Actually, this possibility can be disregarded for a few reasons a few reasons that are explained below.

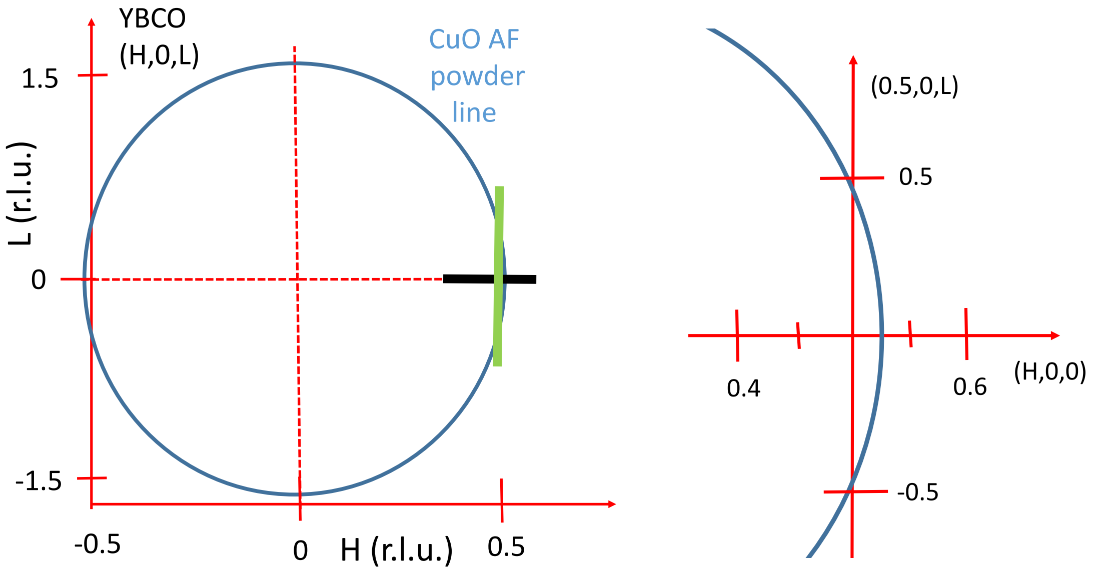


Supplementary Figure S3: Right) Extended (H,0,L) plane of reciprocal space of YBCO. Horizontal black line represents the (H,0,0) scan showing peaks in the manuscript whereas the green one represents the (0.5,0,L) scan. Left) The same (H,0,L) plane zoomed around the (0.5,0,L) region. The H and L directions are properly scaled to each other. In both figures, the blue line represents the trajectory of the CuO antiferromagnetic (-1/2,0 1/2) powder line (projection of the Ewald sphere into the (H,0,L) YBCO plane).

### 2.1 YBCO crystal growth

First, the YBCO69 single crystal was grown at the Shanghai Jiao Tong University. It was obtained by top-seeded solution growth from the Y-Ba-Cu-O solution [3], like ones produced from other flux methods. The solvent has a composition of $Ba_3Cu_5O_y$. The growth temperature is near the peritectic temperature (Tp), which is over 20 K higher than the crystallization temperature for

the solvent material. It means that the solvent material is impossible to form, based on the phase diagram. More importantly, using a very low pulling rate of approximately 0.05 mm/h or less, the growth velocity is less than 1 mm/day along the c-axis direction. Under such a low growth rate, the solvent material is hardly trapped in the crystal. YBCO single crystals grown with this growth technique have already studied with inelastic neutron scattering [4] and quantum oscillations [5] among other techniques. So far, TSSG-processed YBCO single crystal from Shanghai Jiao Tong University have been used by plenty of researchers from physical laboratories worldwide yielding about 20 publications, no CuO impurities contribution was detected and reported.
Further, no intergrowth of CuO in YBCO has ever been documented in approximately 4 decades of studying YBCO. The crystal structure of CuO is monoclinic and its lattice parameters do not match thise of YBCO. Only powdered grains might occur.

### 2.2 Detailed Q-dependence from AF peak of CuO impurities

Second, although the observed magnetic peaks in YBCO69 are not far in Q-space from the one expected from the (1/2,0,-1/2) AF peak of CuO (Fig. S3.a), the perfect matching is actually only at L=1/2 of YBCO not at L=0 (Fig. S3.b). To be accurate, the CuO powder line actually nearly corresponds to the momentum position Q=(1/2,0,1/2) of YBCO which is off in $2\theta$ by 1 deg from Q=(1/2,0,0) on 4F1 for $k_f = 2.57\text{Å}^{-1}$ and by 1.7 deg from Q=(1/2,0,0) on THALES for $k_f = 1.5\text{Å}^{-1}$. As a result, all H-scans for L=0 have to be maximum for H=0.525 in case of a contamination by CuO impurities. We remind that the instrumental $H$-resolution is about $\Delta_q$=0.023 r.l.u. on THALES and $\Delta_q$=0.033 r.l.u. on 4F1 for a powder line. The offset along $H$ from the CuO line would be clearly seen at $L$=0 within the $H$-resolution. Within our experimental conditions, this is clearly not the case in the various figures showing H-scans in the manuscript obtained on two different instruments and two different neutron energies. Next, our signal is larger at L=0 than L=1/2 whereas a smaller intensity would be expected for a contamination by CuO powder impurities due to the $H$ offset. These different points rule out AF contribution from

CuO impurities to explain the observed magnetic peaks.

Next, it has been as well proposed that textured crystallites of CuO (not powder) can account for our neutron diffraction data. However, the observed peaks along $H$ are clearly broader than the $H$ instrumental resolution (longitudinal scan), which means it corresponds to $\sim$ 25 Å nano-size magnetic clusters. Therefore, our measurements are incompatible with CuO crystallites larger than $\sim$ 30 Å in size. To get enough intensity, one then need a large amount of such independent small CuO crystallites in our centimeter size sample, having necessarily random orientations within the YBCO matrix as there is no known intergrowth of CuO in YBCO. Our neutron diffraction data are therefore incompatible with textured crystallites of CuO.

Finally, the double-peak shape reported of the $L$-scan in Fig. 4a of the manuscript precludes that the peaks are coming from CuO powder impurities. That scan is similar to a sample rocking scan: we observe two peaks, not a smooth disappearance with $L$ as expected for a powder contamination. Meanwhile, the Néel temperature $T_N$ of bulk CuO is in the similar range as our report, one then might expect a very sharp magnetic transition at 230K to match the published data in CuO[1]. As shown in Fig. 5, it might be consistent with the temperature dependence of the L=0 peak but not what is observed at L=1/2 where the contamination from the AF peak of CuO is expected to be maximum. However, the Néel temperature of nano-size CuO grains actually drops down drastically with the grain size [6], falling below 50 K when the size is shorter than 50 Å. As only small CuO grains of 25Å size are compatible with our report, their Néel temperature is inconsistent with the reported temperature dependencies of the magnetic scattering at both $L$ (Fig. 5). Finally, the magnetic moment direction in the case of powder impurities has to be simply isotropic in the polarization analysis. No preferential moment direction will be observed contrary to our observations for both $L$=0 and $L$=1/2. Therefore, the details of the reported behaviour of the magnetic peaks are all inconsistent with a contamination from CuO impurities.

### 2.3 Intensity in absolute units from CuO impurities

Third, one can test the existence of possible CuO contaminations by computing the nuclear Bragg peaks spectrum of CuO using the VESTA software, that we report in Fig. S4. It shows as well the comparison of the computed neutron powder spectrum with the measured one in the YBCO69 sample. All powder lines of CuO are included with their calculated Bragg intensities. Clearly, there is no agreement between the expected spectrum and the measured one. In particular, no peaks are observed in the $2\theta$-range of 100 to 120 deg whereas three structural peaks are notably expected from CuO impurities. Further, powder lines (or small grains) from the YBCO structure peaks contribute to peaks at lower $2\theta$ in the range 60 to 75 deg. Consequently, even the weak peak measured at 60 deg cannot be readily attributed to CuO contaminations as all such peaks can be indexed within the YBCO lattice.
To be more quantitative, the contribution from the CuO impurities can be at most 5 counts in the reported powder diffraction spectrum, that typically corresponds to the data error bars in Fig. S4. By comparison with YBCO69 Bragg peaks - in particular the (0,0,4) Bragg peak, that upper limit amounts for only $10^{-5}$. The measured and calculated magnetic peaks intensities from $Cu^{2+}$ spin moments in CuO have been reported in absolute units in ref. [1]. The magnetic form factor has been included as well. It is found that the (1/2,0,-1/2) AF peak is about 20 times weaker than the nuclear peak (1,1,1) (peak at $2\theta \sim 60$ deg in Fig. S4). This indicates that the upper limit of the contribution of the AF peak of CuO is 0.5x$10^{-6}$ of the YBCO69 Bragg intensities.
The observation of the magnetic peak intensity is $\sim$ 8x$10^{-6}$ of the strong YBCO69 Bragg intensities. That number is obtained from the ratio of the (0,0,4) Bragg peak intensity of 20000 cnts/sec measured on 4F1 and the magnetic intensity for the same experiment, reported in Figs. 2b and 4a, which is $\sim$150 cnts in 15 minutes. The upper limit of the calculated intensity from CuO impurities is then at least one order of magnitude too weak to explain the observed magnetic peaks in the YBCO69 sample. CuO impurities can then be readily disregarded to interpret the observed magnetic peaks at $q = 1/2$ in YBCO69.

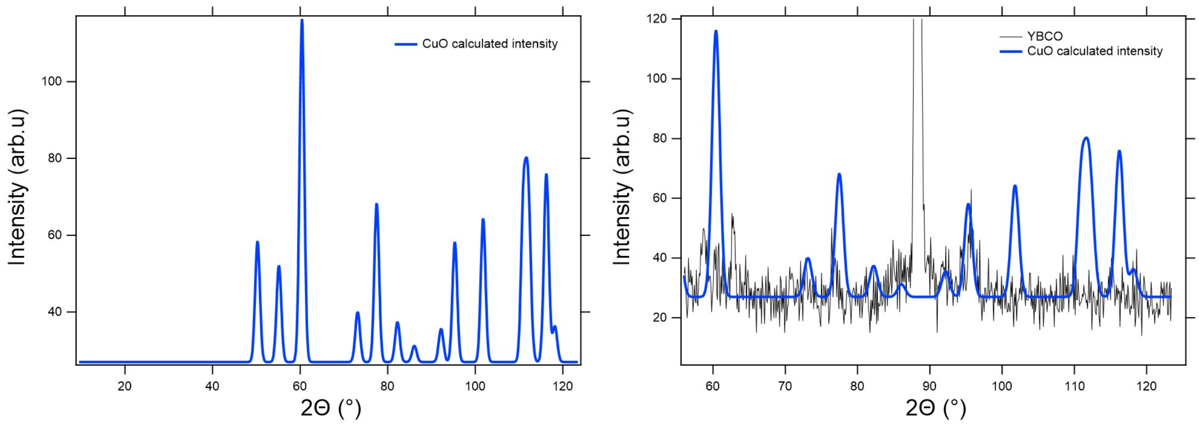


Supplementary Figure S4: Right) Neutron diffraction spectrum from CuO powder computed using the VESTA software. The peaks have been broadened by the convolution by a Gaussian instrumental function with a constant full-width at half maximum of 2 deg. Left) The same computed spectrum compared with the measured powder neutron diffraction spectrum measured in YBCO69 (same as the one shown in Fig. 1c) on the diffractometer 3T1 at the Orphée reactor. The computed intensity is also shifted to match the background level.

# References


[1] Forsyth, J. B., Brown, P. J., and Wanklyn, B. M. *J. Phys. C: Solid State Phys.* **21**, 2917 (1988).

[2] Ain, M., Menelle, A., Wanklyn, B., and Bertaut, E. *J. Phys.: Condens. Matter* **4**, 5227 (1992).

[3] Xiang, H., Guo, L., Li, H., Cui, X., Qian, J., Hussain, G., Liu, Y., Yao, X., Rao, Q., and Zou, Z. *Scripta Materialia* **116**, 36–39 (2016).

[4] Li, S., Yamani, Z., Kang, H. J., Segawa, K., Ando, Y., Yao, X., Mook, H. A., and Dai, P. *Phys. Rev. B* **77**, 014523 Jan (2008).

[5] Singleton, J., de la Cruz, C., McDonald, R. D., Li, S., Altarawneh, M., Goddard, P., Franke, I., Rickel, D., Mielke, C. H., Yao, X., and Dai, P. *Phys. Rev. Lett.* **104**, 086403 Feb (2010).

[6] Zheng, X. G., Xu, C. N., Nishikubo, K., Nishiyama, K., Higemoto, W., Moon, W. J., Tanaka, E., and Otabe, E. S. *Phys. Rev. B* **72**, 014464 Jul (2005).
